# Supplementary material for: The Point-to-Set Principle and the Dimensions of Hamel Bases
Source: arXiv:2109.10981 source file (2023-09-21)
Supplement: Supplementary file 1 [file Appendix.tex]

% !TEX root=../ARCRN.tex
%\section*{Appendix}%% note that this is the original lemma 0.1

%%%% testing
%%\repeattheorem{Ville_thm}
\pagestyle{appendix}
\section{Optional Technical Appendix}
 \setcounter{apthm}{0}

% reset counter
%\setcounter{lemma}{0}
%  \renewcommand{\thelemma}{\Alph{section}\arabic{lemma}}
